# Supplementary material for: Towards understanding the special stability of ${\text{SrCo}\text{O}_{2.5}}$ and ${\text{HSrCo}\text{O}_{2.5}}$
Source: arXiv:1806.03917 ancillary file (2019-02-14)
Supplement: Supplementary file 1 [file 2201_Supplemental.pdf]

# Supplemental Material for *Towards understanding the special stability of $SrCoO_{2.5}$ and $HSrCoO_{2.5}$*


Sze-Chun Tsang, Jingzhao Zhang, Kinfai Tse, and Junyi Zhu*

*Department of Physics, the Chinese University of Hong Kong, Shatin, New Territories, Hong Kong*


## I. MORE ON *U* AND FUNCTIONAL TESTING IN H-SCO

As detailed in the Main Text (MT), a test H-SCO structure (Supp. Fig. 1) was fully relaxed using different sets of functionals (LDA and PBE-GGA), under Hubbard-$U$ values[1] ranging from 0 to 5 eV.

### A. Structural tests

A trend is observed for both functionals that the $a$-lattice vector tends to shorten with increasing $U$, while the $b$-lattice vector lengthened. To examine the data more closely, we take note of the inter-Sr distances in-plane (i.e. in the $b$-, or [010]-direction) and out-of-plane (i.e. in the $a$-, or [100]-direction) (Supp. Fig. 1); they are plotted against $U$ in Supp. Fig. 2.

Compared to the experimental data[2], it is seen that the best fits to the inter-Sr distances are given by LDA, with the optimal $U$ falling somewhere between 1 and 2 eV; however, it is also observed that the LDA distances undergo abrupt changes in that range, which precludes locating the corresponding optimal value. Moreover, as shown in MT Fig. 3(a), the bandgap vanishes in that regime, highlighting the inherent over-estimation of electron delocalization[3] (and subsequently, the metallicity of the system) in LDA.

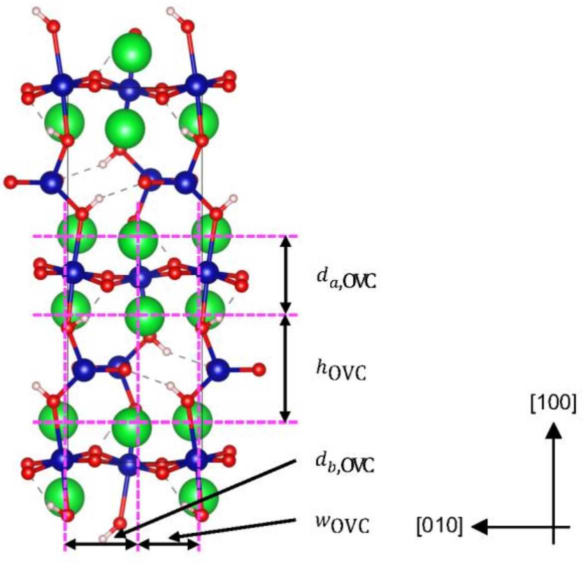


SUPPLEMENTAL FIG. 1. Illustration of the H-SCO test phase, and the four metrics (inter-Sr distances) used to evaluate the match of the relaxed structures with the experimental results: $h_{OVC}$, the OVC "height"; $d_{a,OVC}$, the distance between OVCs in the [100]-direction; $w_{OVC}$, the OVC "width"; and $d_{b,OVC}$, the distance between OVCs in the [010]-direction.

SUPPLEMENTAL TABLE I. Average MM per $Co_{(6)}$ and $Co_{(4)}$ site in the test H-SCO structure obtained at different $U$ values, for both the LDA and PBE-GGA functionals.

| $U$ (eV) | MM ($\mu_B$) | | | |
|---|---|---|---|---|
| | LDA | | PBE-GGA | |
| | $Co_{(6)}$ | $Co_{(4)}$ | $Co_{(6)}$ | $Co_{(4)}$ |
| 0 | 1.07(2) | 1.968(7) | 1.7(6) | 2.272(5) |
| 1 | 1.14(1) | 2.1958(4) | 2.423 | 2.41 |
| 2 | 2.373 | 2.358 | 2.505 | 2.506 |
| 3 | 2.462 | 2.462 | 2.569 | 2.582 |
| 4 | 2.535 | 2.546 | 2.627 | 2.647 |
| 5 | 2.597 | 2.6153(4) | 2.68 | 2.7035(5) |

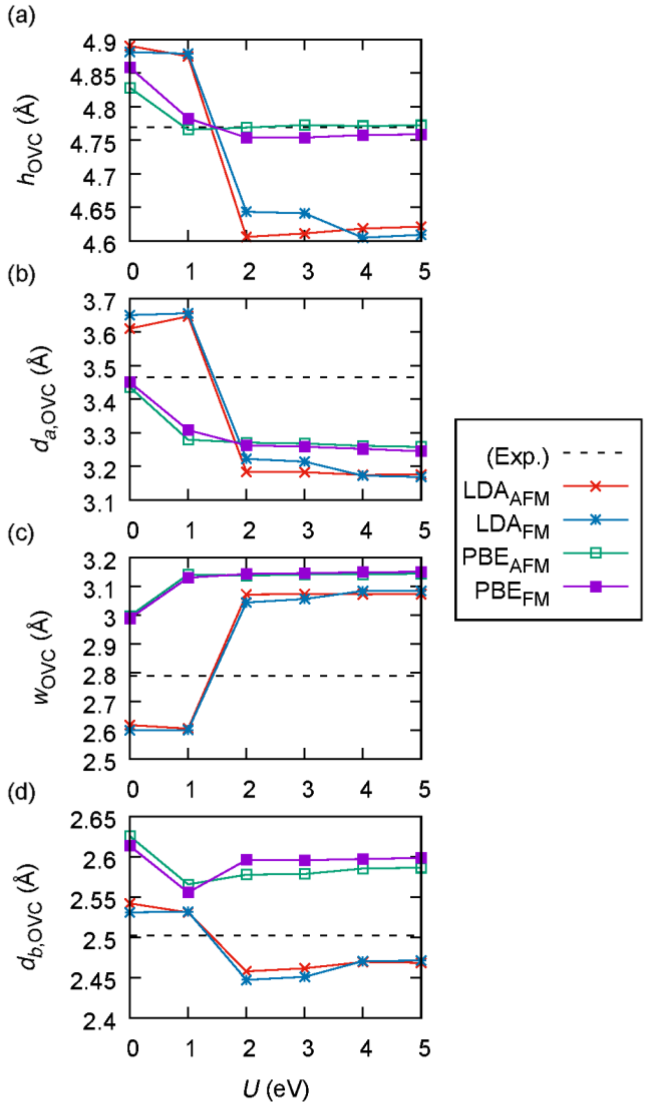


SUPPLEMENTAL FIG. 2. Plot of the inter-Sr distances obtained after relaxations, using the LDA and PBE-GGA, at different $U$ parameters and spin textures. (a) $h_{OVC}$. (b) $d_{a,OVC}$. (c) $w_{OVC}$. (d) $d_{b,OVC}$.

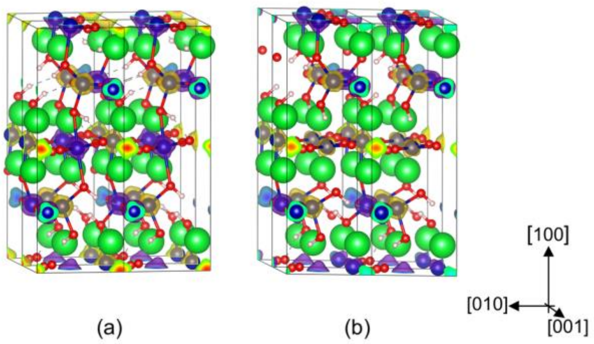


SUPPLEMENTAL FIG. 3. Spin density isosurfaces of the (a) G-type and (b) new AFM spin textures; up and down spins are indicated by gold and purple isosurfaces respectively.

## B. Magnetism-related tests

The magnetic moment (MM) of Co increases steadily with $U$ (Supp. Table I), which is consistent with a depopulation of the minority-spin Co-d levels (MT Fig. 10), caused by the increased energy penalty incurred by paired electrons.

Interestingly, upon relaxation at small values of $U$, the spin texture of H-SCO deviates from the G-type (i.e. checkerboard-like) AFM configuration [Supp. Fig. 3(a)], now consisting of stacked FM-coupled $Co_{(6)}$ layers of opposing spins, interleaved with G-type AFM layers of $Co_{(4)}$–$O_{(4)}$–$Co_{(4)}$ chains [Supp. Fig. 3(b)]. At $U \geq 1$ eV (PBE-GGA) or 2 eV (LDA), the G-type spin texture again becomes energetically favorable. In the LDA cells, such transition is concurrent to the aforementioned (Supp. Fig. 2) drastic change of the structural parameters, and the

SUPPLEMENTAL TABLE II. Comparison between the bandgap and magnetic coupling energies of the test H-SCO structure, obtained using various functionals.

| Energy (eV) | Functional | | |
|---|---|---|---|
| | PBE-GGA | HSE | SCAN |
| $E_g$ | 1.98 | 3.27[a] | 1.52[a] |
| $\Delta F_{AFM-FM}/N_{Co}$ | −0.056 | −0.056 | −0.076 |

[a]Estimated from the eigenvalues sampled on the k-point mesh.

vanishing of the bandgap; whereas in the PBE cell, the new AFM texture still gives a bandgap, albeit unreasonably small [≈ 0.1 eV; rf. MT Fig. 3(a)]. This hints that the new spin texture is unphysical, and may indeed be a mere artefact of the overestimated metallicity.

## C. Results from other functionals

In order to verify the calculated AFM magnetic ground state, two more sample functionals, beside the aforementioned LDA and PBE-GGA, were chosen: from among the "hybrid" functionals, Heyd–Scuseria–Ernzerhof[4] (HSE); and a "meta-GGA" one, the Strongly Constrained and Appropriately Normed [5] (SCAN) functional. Using these two functionals, the H-SCO test cell was again fully relaxed. Relaxation parameters were similar to those documented in Section III A, MT, except that (1) no Hubbard $U$ was imposed; (2) the energy cut-offs were increased (HSE: 450 eV; SCAN: 500 eV); and (3) less-dense 1×3×3 k-point meshes were used.

A comparison of the key results – the bandgap ($E_g$) and magnetic coupling ($\Delta F_{AFM-FM}/N_{Co}$) energies – between the PBE-GGA (with $U = 4$ eV), HSE, and SCAN functionals

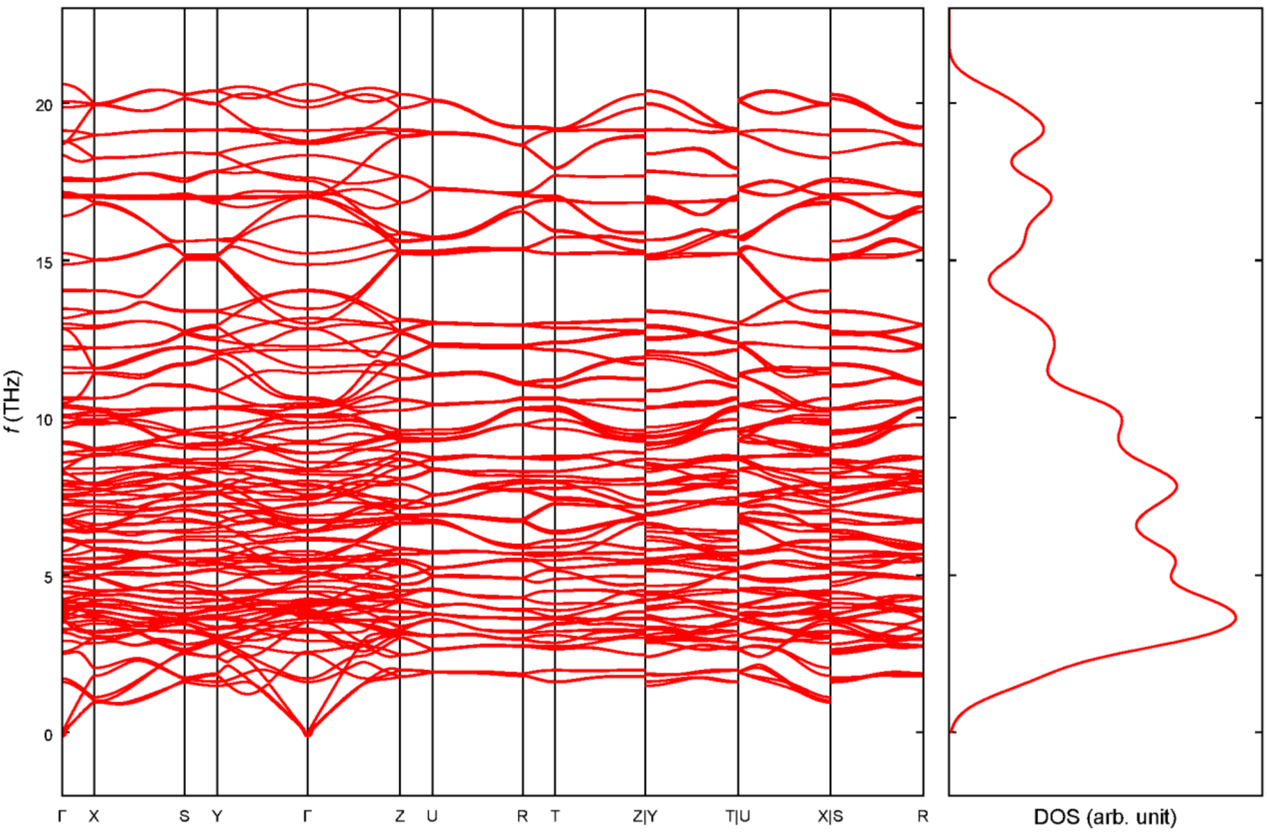


SUPPLEMENTAL FIG. 4. Plots of the phonon band structure (left) and DOS (right) of *phase-1* BM-SCO, where $f$ is the non-angular phonon frequency. Imaginary modes, if any, are mapped to the negative frequencies.

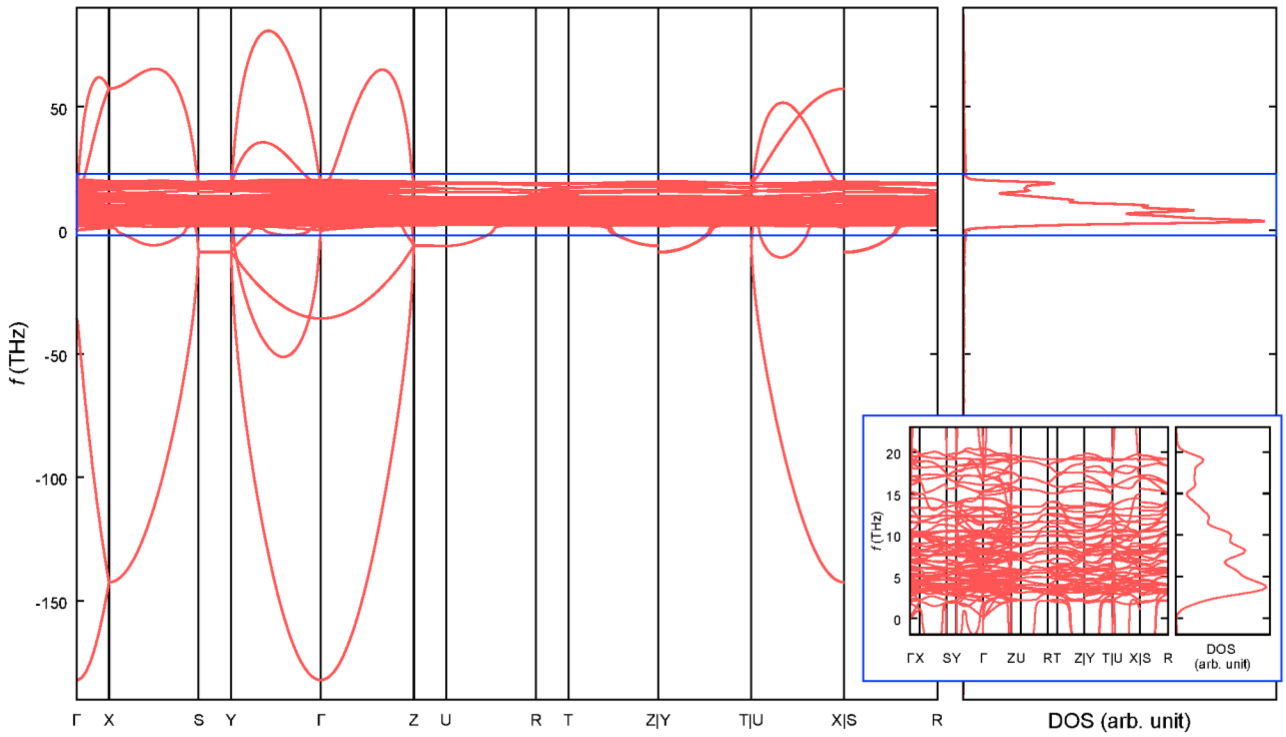


SUPPLEMENTAL FIG. 5. Plots of the phonon band structure (left) and DOS (right) of *phase-3* BM-SCO; conventions follow those in Supp. Fig. 4. Inset: focused view of the frequency range $-2$ THz $< f <$ 23 THz (Enclosed in a blue box in the main Fig.), the same range as in Supp. Fig. 4.

are given in Supp. Table II. As is obvious, the bandgap of H-SCO is consistently large (>1.5 eV), and AFM is found to be energetically favorable across all tested functionals.

## II. PHONON CALCULATIONS ON BM-SCO PHASES

For the analysis of the dynamical stabilities of the obtained BM-SCO phases, phonon spectra were calculated for two phases: *phase 1*, of space group $Pmc2_1$ and of the lowest energy among the obtained phases; and *phase 3*, of the traditionally-attested[6] space group *Ima2*. Calculations were done using VASP[7,8] and *phonopy*[9,10] with the GGA functional, in 144-atom ($2 \times 2 \times 1$) supercells with G-type spin texture on $3 \times 3 \times 2$ Γ-centered k-point meshes. Densities-of-states (DOSes) were obtained by Gaussian smearing with a standard deviation of 0.5 THz.

As shown in Supp. Fig. 4, no imaginary phonon mode was found for *phase 1*, which strongly indicates the $Pmc2_1$ symmetry to be an energy minimum of BM-SCO, at least locally. This is coherent with our experience; the space group arose naturally and consistently in relaxations. In contrast, the spectrum of the more-symmetric *phase 3* is riddled with imaginary modes (Supp. Fig. 5) – a sign of dynamical instability. Though the DOSes of the two phases (Supp. Fig. 4, 5 inset) are seemingly similar within the focused range, the two spectra differ greatly in the high- and imaginary-frequency domains.

## III. ADDITIONAL INFORMATION ON THE SINGLE-HYDROGEN CONFIGURATIONS

Beside simplistic energetic comparisons of the single-H configurations (MT Fig. 7), it is also instructive to look at the changes to the electronic and magnetic structures of BM-SCO induced by the hydrogenation. As shown in Supp. Table III (data previously presented by Tsang[11]), the semiconductivity of BM-SCO is preserved under the light H-doping, with narrower gaps compared to the no-H case [1.37 eV (MT Table II)]. Also, owing to the partial injection of the electron from H into the system (rf. Section IV B 2, MT), in each of the single-H configurations, there is

SUPPLEMENTAL TABLE III. Additional information (based on [11]) on the single-H configurations. Bandgap energies are estimated from the eigenvalues sampled on the k-point mesh.

| Configuration | $E_g$ estimate (eV) | Co site w/ decreased MM | | Average MM of other Co sites ($\mu_B$) | |
|---|---|---|---|---|---|
| | | $Co_{(6)}$ or $Co_{(4)}$ | MM ($\mu_B$) | $Co_{(6)}$ | $Co_{(4)}$ |
| $O_{(Sr)}$–$O_{(6)}$-away | 1.05 | $Co_{(6)}$ | 2.538 | 2.95(1) | 2.862(5) |
| $O_{(6)}$–$O_{(Sr)}$-away | 1.29 | $Co_{(6)}$ | 2.571 | 2.955(5) | 2.863(4) |
| $O_{(6)}$–$O_{(Sr)}$-towards | 1.26 | $Co_{(6)}$ | 2.564 | 2.954(6) | 2.861(4) |
| $O_{(4)}$-along | 0.95 | $Co_{(6)}$ | 2.535 | 2.955(6) | 2.86(2) |
| $O_{(4)}$-across | 1.27 | $Co_{(4)}$ | 2.526 | 2.955(4) | 2.863(6) |
| $O_{(Sr)}$–$O_{(4)}$-across | 1.03 | $Co_{(6)}$ | 2.544 | 2.952(9) | 2.860(4) |
| Mid-OVC | 1.01 | $Co_{(4)}$ | 2.325 | 2.955(1) | 2.861(4) |
| Wall-OVC | 1.00 | $Co_{(4)}$ | 2.361 | 2.9554(8) | 2.861(4) |

consistently one single Co site with a significantly decreased MM, while the MMs of the remaining Co sites [2.959 $\mu_B$ ($Co_{(6)}$) and 2.915 $\mu_B$ ($Co_{(4)}$); rf. MT Table II] in the simulation cell remain relatively unchanged. These two facts show how the perturbation to the system due to the H atom is localized, and the hopping of the H-electron limited.

With the locality of the effects of sparse interstitial H atoms established, the interactions between more of them, as would arise when the H concentration is increased, are also expected to be limited. Hence, we can with greater confidence construct fully-hydrogenated structures (MT Fig. 8) from the sampled single-H local configurations, without the explicit sampling of configurations in the intermediately-hydrogenated regime.

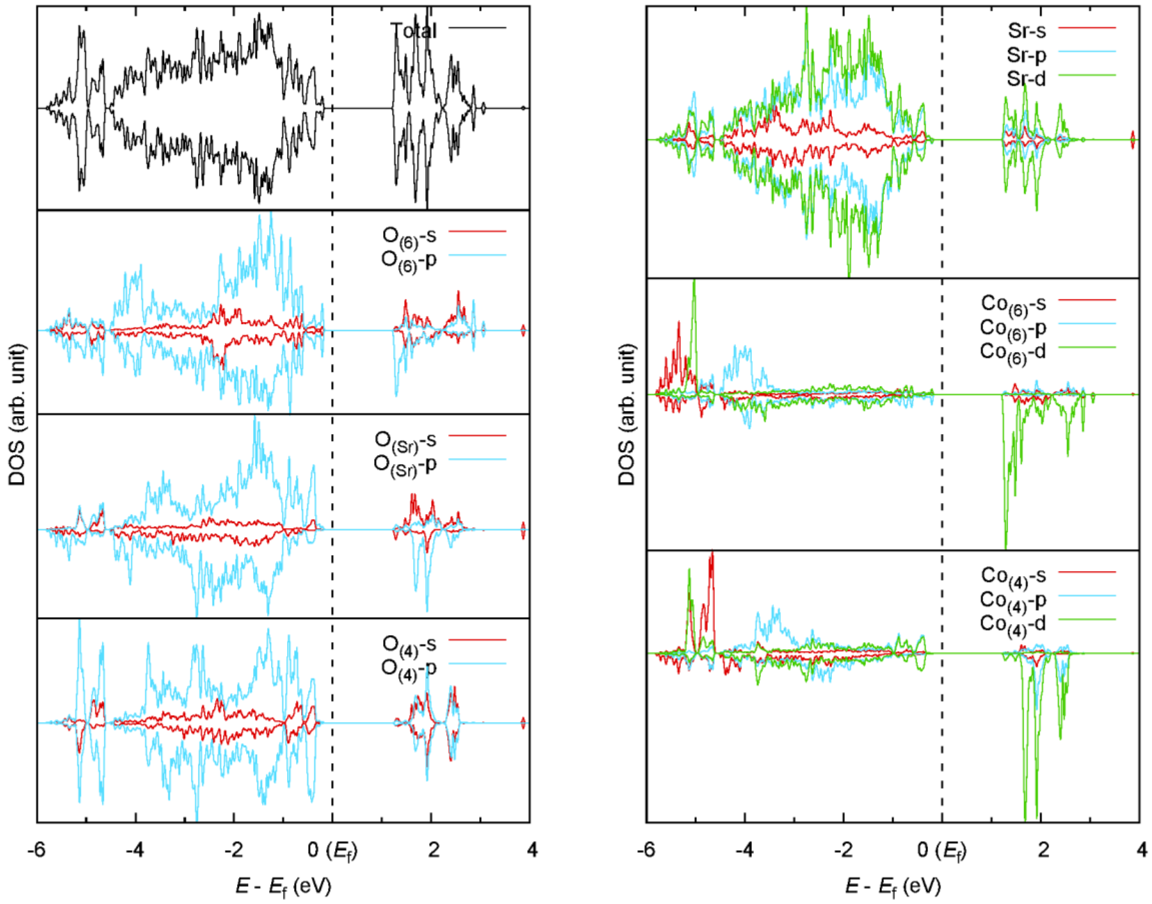


SUPPLEMENTAL FIG. 6. Plots of the projected DOSes (pDOSes) in *phase-1* BM-SCO.

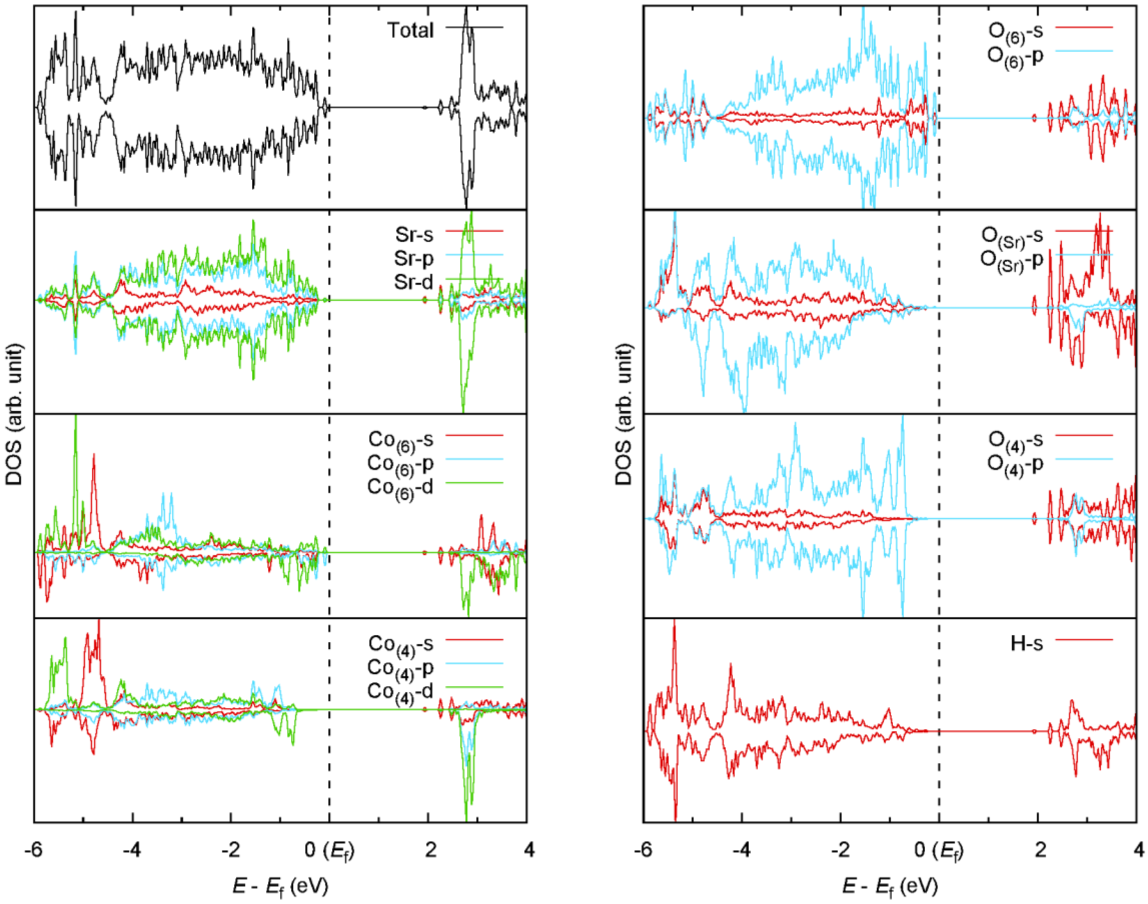


SUPPLEMENTAL FIG. 7. Plots of the pDOSes in H-SCO.

## IV. BAND COMPONENT ANALYSES OF THE MAJOR PHASES DISCUSSED

For detailed analyses of the electronic structures of BM-SCO and H-SCO, we also provide hereby projected DOSes (pDOSes; Supp. Fig. 6, 7) and band-structure plots with $l$-resolved projections (Supp. Fig. 8–10).

[In the subsequent discussion, the reader is referred to the more transparent band-structure plots; the pDOSes are provided only for completeness, and for easy comparison with literature.[2,6] In the band-structure plots, the $l$-resolved species projections at each sampled k-point on each band are visualized by translucent circles (spin-up: red; spin-down: blue). The area of each circle is proportional to the projection in question, normalized by the sum of all projections made by VASP on that band at that k-point.]

For *phase-1* BM-SCO, the conduction band (CB) is predominantly attributable to the $Co_{(6)}$-d and $O_{(6)}$-p orbitals

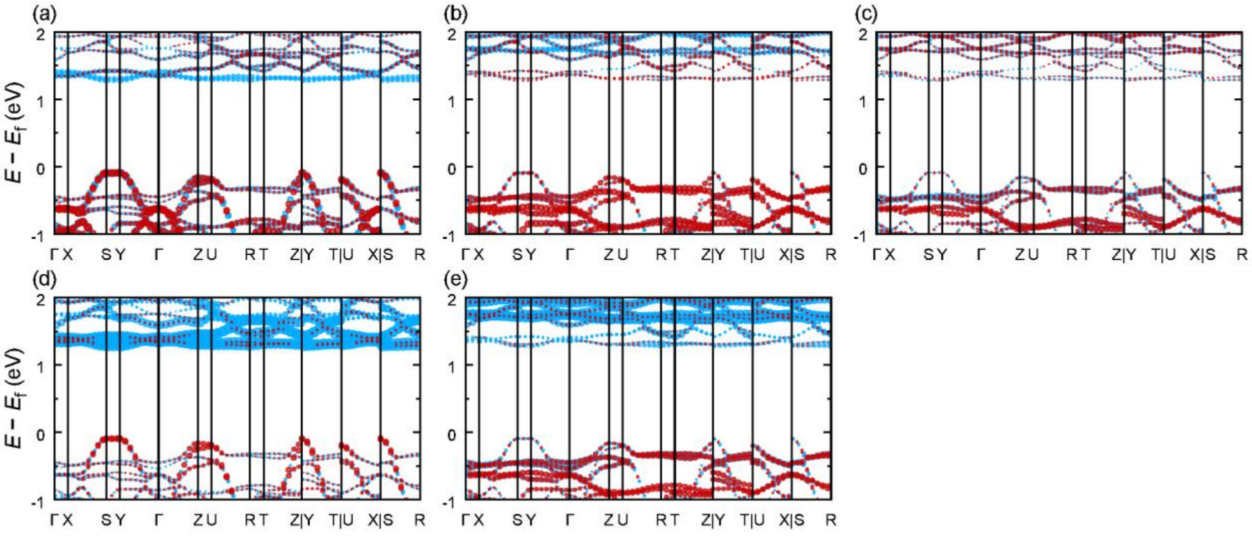


SUPPLEMENTAL FIG. 8. Plots of the $l$-resolved species projections onto the band structure of *phase-1* BM-SCO near the band edges. In respective order: (a) $O_{(6)}$-p. (b) $O_{(Sr)}$-p. (c) $O_{(4)}$-p. (d) $Co_{(6)}$-d. (e) $Co_{(4)}$-d.

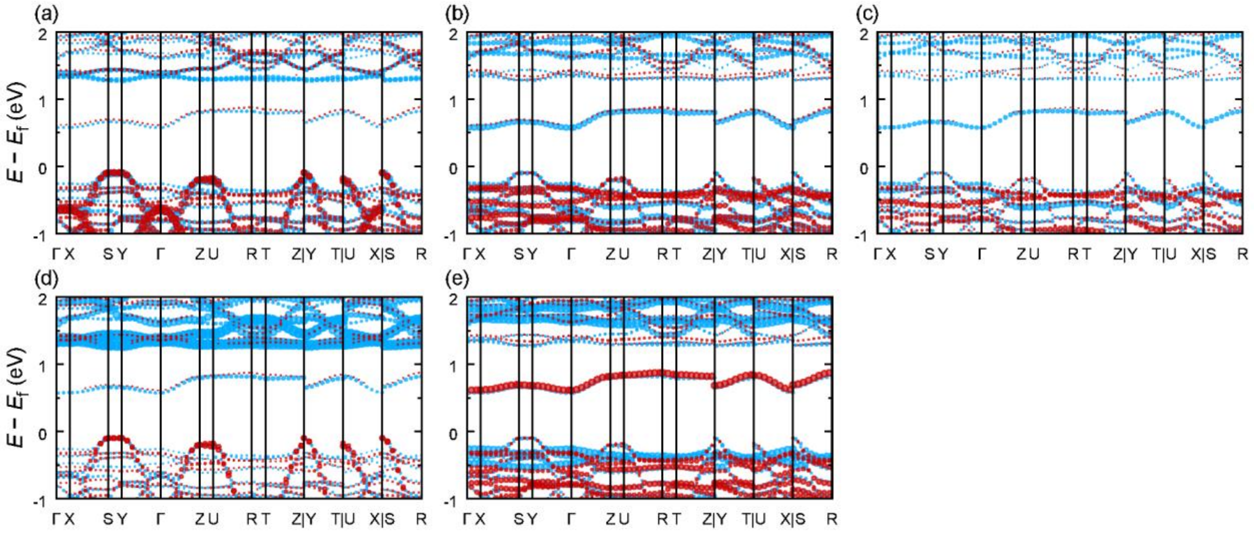


SUPPLEMENTAL FIG. 9. Plots of the *l*-resolved species projections onto the band structure of *phase-2* BM-SCO near the band edges. In respective order: (a) $O_{(6)}$-p. (b) $O_{(Sr)}$-p. (c) $O_{(4)}$-p. (d) $Co_{(6)}$-d. (e) $Co_{(4)}$-d. Note especially gap state created, relative to *phase 1* (Supp. Fig. 8).

[Supp. Fig. 8(a), (d)]. Meanwhile, the valence band (VB) is more complicated: near the VB top, around the Y, Z, S, and U points, the VB is of similar character to the CB, except that it has a little $Co_{(6)}$-p character; however, contributions from $Co_{(4)}$-d, $O_{(Sr)}$-p, and $O_{(4)}$-p orbitals dominate mid-VB and near the VB bottom [Supp. Fig. 8(b), (c), (e)]. In *phase-2* BM-SCO, due to the break of symmetry (MT Table II), a gap state of substantial $Co_{(4)}$–$O_{(Sr)}$ nature [Supp. Fig. 9(b), (e)] is created, while leaving the original VB, CB, and their band components largely intact.

As for H-SCO, the CB is shown to be significantly hybridized, with comparable contributions from a myriad of orbitals. In particular, the CB minimum (CBM) at the Γ point has contributions from, for example, Sr- and Co-s [Supp. Fig. 10(g–i)], Co-d [Supp. Fig. 10(e), (f)], as well as the various O orbitals [Supp. Fig. 10(a–d)]. Further away from the Γ point, the CB becomes predominantly Co-d in character [Supp. Fig. 10(e), (f)], with some coupling to O states [Supp. Fig. 10(a–d)]. In comparison, the whole VB is of a definite $Co_{(6)}$-d and $O_{(6)}$-p signature [Supp. Fig. 10(a), (e)], with the $Co_{(4)}$-d and $O_{(4)}$-p states shifting further down

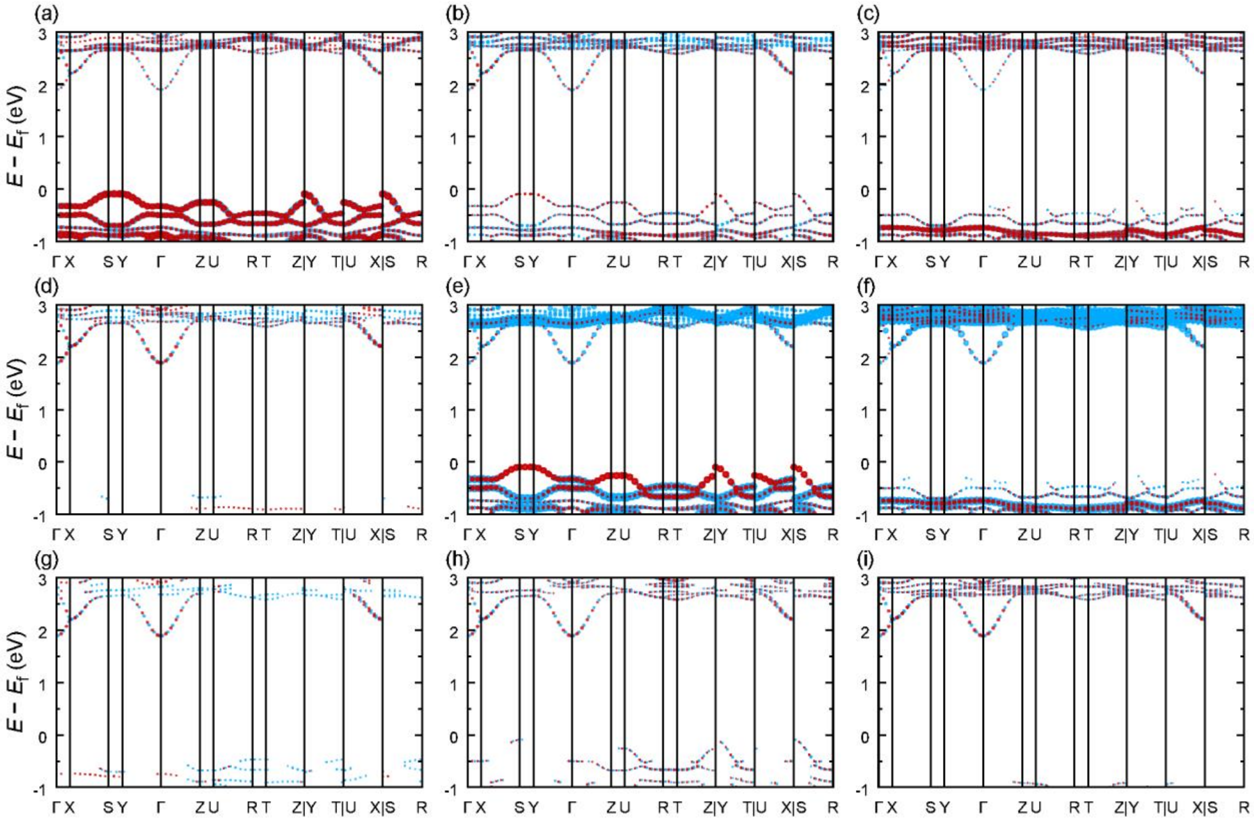


SUPPLEMENTAL FIG. 10. Plots of the *l*-resolved species projections onto the band structure of H-SCO near the band edges. In respective order: (a) $O_{(6)}$-p. (b) $O_{(Sr)}$-p. (c) $O_{(4)}$-p. (d) $O_{(Sr)}$-s. (e) $Co_{(6)}$-d. (f) $Co_{(4)}$-d. (g) Sr-s. (h) $Co_{(6)}$-s. (i) $Co_{(4)}$-s.

into the filled bands [Supp. Fig. 10(c), (f)] – as opposed to the VB in BM-SCO, where tetrahedral-layer contributions are also significant [Supp. Fig. 8(c), (e)].

## V. INFORMATION FOR THE DISCUSSED STRUCTURES

Four structures are hereby disclosed: the *phase-1* (space group $Pmc2_1$), *-2* (slightly monoclinic), and *-3* (space group *Ima2*) BM-SCO structures, and the most-stable H-SCO structure. The fully-relaxed structures are imported as VASP-native `POSCAR` files, and converted into `.cif` files using Python Materials Genomics (*pymatgen*) [12] at a tolerance (`symprec`) of 0.05 for determining equivalent positions.

*Phase-1* BM-SCO:

```
# generated using pymatgen
data_Sr2Co2O5
_symmetry_space_group_name_H-M   Pmc2_1
_cell_length_a   15.58936266
_cell_length_b   5.56971023
_cell_length_c   5.43751103
_cell_angle_alpha   90.00000000
_cell_angle_beta   90.00000000
_cell_angle_gamma   90.00000000
_symmetry_Int_Tables_number   26
_chemical_formula_structural   Sr2Co2O5
_chemical_formula_sum   'Sr8 Co8 O20'
_cell_volume   472.12947296
_cell_formula_units_Z   4
loop_
 _symmetry_equiv_pos_site_id
 _symmetry_equiv_pos_as_xyz
  1  'x, y, z'
  2  '-x, -y, z+1/2'
  3  '-x, y, z'
  4  'x, -y, z+1/2'
loop_
 _atom_site_type_symbol
 _atom_site_label
 _atom_site_symmetry_multiplicity
 _atom_site_fract_x
 _atom_site_fract_y
 _atom_site_fract_z
 _atom_site_occupancy
  Sr  Sr1  4  0.138531  0.260433  0.986294  1
  Sr  Sr2  4  0.361094  0.238348  0.987031  1
  Co  Co3  4  0.249948  0.250570  0.482302  1
  Co  Co4  2  0.000000  0.191232  0.513591  1
  Co  Co5  2  0.500000  0.310341  0.516687  1
  O  O6  4  0.108866  0.295455  0.468611  1
  O  O7  4  0.242785  0.011478  0.247901  1
  O  O8  4  0.256869  0.484153  0.722459  1
  O  O9  4  0.391058  0.206347  0.470789  1
  O  O10  2  0.000000  0.112286  0.853189  1
  O  O11  2  0.500000  0.386122  0.856513  1
```

*Phase-2* BM-SCO:

```
# generated using pymatgen
data_Sr2Co2O5
_symmetry_space_group_name_H-M   Pm
_cell_length_a   5.44026762
_cell_length_b   15.63615408
_cell_length_c   5.53365700
_cell_angle_alpha   90.00000000
_cell_angle_beta   90.86072659
_cell_angle_gamma   90.00000000
_symmetry_Int_Tables_number   6
_chemical_formula_structural   Sr2Co2O5
_chemical_formula_sum   'Sr8 Co8 O20'
_cell_volume   470.66665884
_cell_formula_units_Z   4
loop_
 _symmetry_equiv_pos_site_id
 _symmetry_equiv_pos_as_xyz
  1  'x, y, z'
  2  'x, -y, z'
loop_
 _atom_site_type_symbol
 _atom_site_label
 _atom_site_symmetry_multiplicity
 _atom_site_fract_x
 _atom_site_fract_y
 _atom_site_fract_z
 _atom_site_occupancy
  Sr  Sr1  2  0.485876  0.361894  0.012748  1
  Sr  Sr2  2  0.488565  0.139566  0.991137  1
  Sr  Sr3  2  0.984909  0.138068  0.512250  1
  Sr  Sr4  2  0.988434  0.360312  0.489627  1
  Co  Co5  2  0.482998  0.251091  0.504534  1
  Co  Co6  2  0.983840  0.247582  0.003308  1
  Co  Co7  1  0.007023  0.500000  0.931442  1
  Co  Co8  1  0.021921  0.000000  0.065419  1
  Co  Co9  1  0.505986  0.000000  0.433929  1
  Co  Co10  1  0.522833  0.500000  0.565432  1
  O  O11  2  0.223766  0.256457  0.769096  1
  O  O12  2  0.248510  0.244351  0.264074  1
  O  O13  2  0.463070  0.107562  0.541855  1
  O  O14  2  0.475692  0.389885  0.465994  1
  O  O15  2  0.724814  0.254235  0.738495  1
  O  O16  2  0.748684  0.243871  0.242240  1
  O  O17  2  0.964104  0.392137  0.038451  1
  O  O18  2  0.974912  0.110113  0.965310  1
  O  O19  1  0.344096  0.500000  0.850240  1
  O  O20  1  0.359693  0.000000  0.114293  1
  O  O21  1  0.842200  0.000000  0.349506  1
  O  O22  1  0.861462  0.500000  0.611481  1
```

*Phase-3* BM-SCO:

```
# generated using pymatgen
data_Sr2Co2O5
_symmetry_space_group_name_H-M   Ima2
_cell_length_a   15.52857381
_cell_length_b   5.60176355
_cell_length_c   5.40177719
_cell_angle_alpha   90.00000000
_cell_angle_beta   90.00000000
_cell_angle_gamma   90.00000000
_symmetry_Int_Tables_number   46
_chemical_formula_structural   Sr2Co2O5
_chemical_formula_sum   'Sr8 Co8 O20'
_cell_volume   469.88654663
_cell_formula_units_Z   4
loop_
 _symmetry_equiv_pos_site_id
 _symmetry_equiv_pos_as_xyz
  1  'x, y, z'
  2  '-x, -y, z'
  3  '-x+1/2, y, z'
  4  'x+1/2, -y, z'
  5  'x+1/2, y+1/2, z+1/2'
  6  '-x+1/2, -y+1/2, z+1/2'
  7  '-x, y+1/2, z+1/2'
  8  'x, -y+1/2, z+1/2'
loop_
 _atom_site_type_symbol
 _atom_site_label
 _atom_site_symmetry_multiplicity
 _atom_site_fract_x
 _atom_site_fract_y
 _atom_site_fract_z
 _atom_site_occupancy
  Sr  Sr1  8  0.110722  0.011357  0.495335  1
  Co  Co2  4  0.000000  0.000000  0.000000  1
  Co  Co3  4  0.250000  0.559867  0.467479  1
  O  O4  8  0.006883  0.747765  0.245199  1
  O  O5  8  0.140439  0.043452  0.010847  1
  O  O6  4  0.250000  0.637517  0.125843  1
```

H-SCO:

```
# generated using pymatgen
data_Sr2Co2H2O5
_symmetry_space_group_name_H-M   Pna2_1
_cell_length_a   16.06417237
_cell_length_b   5.72660078
_cell_length_c   5.62640983
_cell_angle_alpha   90.00000000
_cell_angle_beta   90.00000000
_cell_angle_gamma   90.00000000
_symmetry_Int_Tables_number   33
_chemical_formula_structural   Sr2Co2H2O5
_chemical_formula_sum   'Sr8 Co8 H8 O20'
_cell_volume   517.59089386
_cell_formula_units_Z   4
loop_
 _symmetry_equiv_pos_site_id
 _symmetry_equiv_pos_as_xyz
  1  'x, y, z'
  2  '-x, -y, z+1/2'
  3  '-x+1/2, y+1/2, z+1/2'
  4  'x+1/2, -y+1/2, z'
loop_
 _atom_site_type_symbol
 _atom_site_label
 _atom_site_symmetry_multiplicity
 _atom_site_fract_x
 _atom_site_fract_y
 _atom_site_fract_z
 _atom_site_occupancy
  Sr  Sr1  4  0.140749  0.322617  0.965871  1
  Sr  Sr2  4  0.156149  0.775463  0.430656  1
  Co  Co3  4  0.003545  0.129651  0.552699  1
  Co  Co4  4  0.244189  0.291008  0.459701  1
  H  H5  4  0.044700  0.488352  0.395464  1
  H  H6  4  0.133596  0.877376  0.861587  1
  O  O7  4  0.001695  0.827413  0.393058  1
  O  O8  4  0.085987  0.361099  0.415458  1
  O  O9  4  0.109473  0.751679  0.960377  1
  O  O10  4  0.223627  0.046008  0.712955  1
  O  O11  4  0.245309  0.048850  0.204140  1
```

[*] Corresponding author; jyzhu@phy.cuhk.edu.hk

[1] J. Hubbard, Proc. R. Soc. A **276**, 238 (1963).
[2] N. Lu, P. Zhang, Q. Zhang, R. Qiao, Q. He, H.-B. Li, Y. Wang, J. Guo, D. Zhang, Z. Duan, Z. Li, M. Wang, S. Yang, M. Yan, E. Arenholz, S. Zhou, W. Yang, L. Gu, C.-W. Nan, J. Wu, Y. Tokura, and P. Yu, Nature **546**, 124 (2017).
[3] P. Mori-Sánchez, A. J. Cohen, and W. Yang, Phys. Rev. Lett. **100**, 146401 (2008).
[4] J. Heyd, G. E. Scuseria, and M. Ernzerhof, J. Chem. Phys. **118**, 8207 (2003); **124**, 219906(E) (2006).
[5] J. Sun, A. Ruzsinszky, and J. P. Perdew, Phys. Rev. Lett. **115**, 036402 (2015).
[6] A. Muñoz, C. de la Calle, J. A. Alonso, P. M. Botta, V. Pardo, D. Baldomir, and J. Rivas, Phys. Rev. B **78**, 054404 (2008).
[7] G. Kresse and J. Furthmüller, Comput. Mater. Sci. **6**, 15 (1996).
[8] G. Kresse and J. Furthmüller, Phys. Rev. B **54**, 11169 (1996).
[9] A. Togo, F. Oba, and I. Tanaka, Phys. Rev. B **78**, 134106 (2008).
[10] A. Togo, F. Oba, and I. Tanaka, Scr. Mater. **108**, 1 (2015).
[11] S.-C. Tsang, M.Phil. thesis, The Chinese University of Hong Kong, 2018.
[12] S. P. Ong, W. D. Richards, A. Jain, G. Hautier, M. Kocher, S. Cholia, D. Gunter, V. L. Chevrier, K. A. Persson, and G. Ceder, Comput. Mater. Sci. **68**, 314 (2013).
